# Supplementary material for: Time-dependent density functional theory of high excitations: To infinity, and beyond
Source: arXiv:0901.3418 source file (2009-02-11)
Supplement: Supplementary file 1 [file table_supplement.pdf]

TABLE I: The  $\mu_i$  for the He atom figures in the paper “Time-dependent density functional theory of high excitations: To infinity, and beyond” by Meta van Faassen and Kieron Burke. The coefficients fit the quantum defect and  $\pi$  times the phase shift. The ionization energies are in [a.u.]. The reference results are from Ref. [1].

|                 |         | $s$     |         |           | $p$     |         |           |
|-----------------|---------|---------|---------|-----------|---------|---------|-----------|
|                 |         | EXX     | Exact   | Reference | EXX     | Exact   | Reference |
| $I$             |         | 0.9179  | 0.9037  | 0.9037    |         |         |           |
| KS              | $\mu_0$ | 0.2167  | 0.2135  |           | 0.0232  | 0.0162  |           |
|                 | $\mu_1$ | -0.0404 | -0.0377 |           | 0.0280  | 0.0241  |           |
|                 | $\mu_2$ | 0.0095  | 0.0071  |           | -0.0183 | -0.0097 |           |
|                 | $\mu_3$ |         |         |           | 0.0066  | 0.0019  |           |
| Singlet Hartree | $\mu_0$ |         | 0.0531  | 0.1399    |         | -0.0803 | -0.0120   |
|                 | $\mu_1$ |         | -0.0415 | -0.0528   |         | -0.0270 | -0.0146   |
|                 | $\mu_2$ |         | 0.0698  | 0.0358    |         | 0.0815  | 0.0343    |
|                 | $\mu_3$ |         | -0.0310 |           |         | -0.0393 | -0.0139   |
| Singlet EXX     | $\mu_0$ |         | 0.1196  | 0.1399    |         | -0.0383 | -0.0120   |
|                 | $\mu_1$ |         | -0.0081 | -0.0528   |         | 0.0064  | -0.0146   |
|                 | $\mu_2$ |         | 0.0078  | 0.0358    |         | 0.0372  | 0.0343    |
|                 | $\mu_3$ |         |         |           |         | -0.0210 | -0.0139   |
| Triplet EXX     | $\mu_0$ |         | 0.3432  | 0.2967    |         | 0.0918  | 0.0682    |
|                 | $\mu_1$ |         | -0.1851 | -0.0764   |         | 0.0041  | 0.0365    |
|                 | $\mu_2$ |         | 0.1499  | 0.0167    |         | -0.0297 | -0.0477   |
|                 | $\mu_3$ |         | -0.0630 |           |         | 0.0173  | 0.0206    |
| Singlet ALDAx   | $\mu_0$ |         | 0.1074  | 0.1399    |         |         |           |
|                 | $\mu_1$ |         | -0.0372 | -0.0528   |         |         |           |
|                 | $\mu_2$ |         | 0.0860  | 0.0358    |         |         |           |
|                 | $\mu_3$ |         | -0.0446 |           |         |         |           |
| Triplet ALDAx   | $\mu_0$ |         | 0.3043  | 0.2967    |         |         |           |
|                 | $\mu_1$ |         | -0.1109 | -0.0764   |         |         |           |
|                 | $\mu_2$ |         | 0.0910  | 0.0167    |         |         |           |
|                 | $\mu_3$ |         | -0.0411 |           |         |         |           |
| Singlet ALDA    | $\mu_0$ | 0.1154  | 0.1114  | 0.1399    |         | 0.0007  | -0.0120   |
|                 | $\mu_1$ | -0.0545 | -0.0539 | -0.0528   |         | -0.0992 | -0.0146   |
|                 | $\mu_2$ | 0.1074  | 0.1090  | 0.0358    |         | 0.1947  | 0.0343    |
|                 | $\mu_3$ | -0.0547 | -0.0560 |           |         | -0.1005 | -0.0139   |
| Triplet ALDA    | $\mu_0$ | 0.2754  | 0.2728  | 0.2967    |         | 0.0731  | 0.0682    |
|                 | $\mu_1$ | -0.0655 | -0.0658 | -0.0764   |         | -0.0042 | 0.0365    |
|                 | $\mu_2$ | 0.0188  | 0.0190  | 0.0167    |         | 0.0108  | -0.0477   |
|                 | $\mu_3$ |         |         |           |         | -0.0064 | 0.0206    |
| Singlet hybrid  | $\mu_0$ |         | 0.1265  | 0.1399    |         | -0.0273 | -0.0120   |
|                 | $\mu_1$ |         | -0.0271 | -0.0528   |         | -0.0187 | -0.0146   |
|                 | $\mu_2$ |         | 0.0440  | 0.0358    |         | 0.0755  | 0.0343    |
|                 | $\mu_3$ |         | -0.0227 |           |         | -0.0417 | -0.0139   |
| Triplet hybrid  | $\mu_0$ |         | 0.3240  | 0.2967    |         | 0.0644  | 0.0682    |
|                 | $\mu_1$ |         | -0.1409 | -0.0764   |         | 0.0541  | 0.0365    |
|                 | $\mu_2$ |         | 0.0549  | 0.0167    |         | -0.1043 | -0.0477   |
|                 | $\mu_3$ |         |         |           |         | 0.0572  | 0.0206    |

- 
- [1] G. W. F. Drake in *Atomic, Molecular, and Optical Physics Handbook*, ed. G. W. F. Drake; AIP Press, Woodbury, NY, 1996; p. 154.
